# Supplementary material for: Nonreciprocal collective magnetostatic wave modes in geometrically asymmetric bilayer structure with nonmagnetic spacer
Source: arXiv:2210.14882 ancillary file (2023-03-19)
Supplement: Supplementary file 1 [file Suppl_Mat.pdf]

# Nonreciprocal collective magnetostatic wave modes in geometrically asymmetric bilayer structure with nonmagnetic spacer: Supplementary Materials

P. I. Gerevenkov,* A. M. Kalashnikova, and N. E. Khokhlov
*Ioffe Institute, 194021 St. Petersburg, Russia*

V. D. Bessonov, V. S. Teplov, and A. V. Telegin
*M.N. Mikheev Institute of Metal Physics,*
*UB of RAS, 620108 Ekaterinburg, Russia*

(Dated: March 6, 2023)

## I. METHOD DETAILS

To determine the frequencies of magnetization dynamics we use Landau-Lifshitz eqation considering effective internal magnetic field and exchange interaction away from the borders:

$$\frac{1}{|\gamma|\mu_0}\frac{\partial \mathbf{M}}{\partial t} = -\mathbf{M}\times\left[\mathbf{H} + \frac{2A}{\mu_0 M_S^2}\Delta\mathbf{M}\right], \tag{S.1}$$

and Maxwell equations:

$$\begin{aligned} &\nabla\times\mathbf{H} = 0, \\ &\nabla\cdot\left(\mu_0\left[\mathbf{H}+\mathbf{M}\right]\right) = 0, \end{aligned} \tag{S.2}$$

where $\mathbf{M}$ – magnetization vector, $\mathbf{H}$ – effective magnetic field vector, containing external field and magnetocrystalline anisotropy contributions, $\gamma = 1.76\ 10^{11}\ \frac{rad}{sT}$ is the giromagnetic ratio, $M_S$ – saturation magnetization, $A$ – exchange stiffness, $\mu_0$ – permeability of vacuum, $\Delta$ – Laplace operator and $\nabla$ – nabla-operator.

Directing the X axis along the effective field and separating the time-dependent and time-independent parts under the assumption of small deviations, we obtain: $\mathbf{H} = \{H_{eff}, 0, 0\} + \{0, h_y, h_z\}$ and $\mathbf{M} = \{M_S, 0, 0\} + \{0, m_y, m_z\}$. The $m_j$ and $h_j$, where j means y or z components has the form:

$$\begin{aligned} &\text{inside the ferromagnetic layer} \\ &\begin{cases} m_j = m_{0j}E^{i(\omega t - k_x x - s_y|k_y|y - k_z z)} \\ h_j = h_{0j}E^{i(\omega t - k_x x - s_y|k_y|y - k_z z)} \end{cases} \\ &\text{and outside the ferromagnetic layer} \\ &\begin{cases} m_j^e = 0 \\ h_j^e = h_{0j}^e E^{i(\omega t - k_x x - s_y|k_y|y - k_z^e z)} \end{cases} \end{aligned} \tag{S.3}$$

where $m_{0j}$, $h_{0j}$ and $h_{0j}^e$ – corresponding complex amplitudes, $i$ – imaginary unit, $\omega = 2\pi f$ is the frequency of magnetization dynamics, $k_x, k_y$ and $k_z$ – components of wave vector and $s_y$ is the sign of $k_y$.

* petr.gerevenkov@mail.ioffe.ru; http://www.ioffe.ru/ferrolab/

Using S.1, S.2 and S.3 we obtain dispersion without taking into account the boundary conditions:

$$\left(\frac{2A}{\mu_0 M_S}k^2 + H_{eff}\right)\left(\frac{2A}{\mu_0 M_S}k^4 + H_{eff}k^2 + M_S(k_z^2 + k_y^2)\right) - \frac{\omega^2}{\mu_0^2\gamma^2}k^2 = 0, \tag{S.4}$$

where $k^2 = k_x^2 + k_y^2 + k_z^2$.

Consider waves propagating perpendicular to the external field $k_x = 0$. Then 6 solutions inside the ferromagnetic layer for $k_z$ have the form:

$$\begin{aligned} k_{z1} &= -k_{z2} = ik_y, \\ k_{z3} &= -k_{z4} = i\sqrt{{k_y}^2 + \frac{M_S}{2A}\left[\mu_0 H_{eff} + \frac{1}{2}\mu_0 M_S + \sqrt{\left(\frac{1}{2}\mu_0 M_S\right)^2 + \left(\frac{\omega}{\gamma}\right)}\right]}, \\ k_{z5} &= -k_{z6} = i\sqrt{{k_y}^2 + \frac{M_S}{2A}\left[\mu_0 H_{eff} + \frac{1}{2}\mu_0 M_S - \sqrt{\left(\frac{1}{2}\mu_0 M_S\right)^2 + \left(\frac{\omega}{\gamma}\right)}\right]} \end{aligned} \tag{S.5}$$

Now consider the condition on the interfaces. Following [1–3], we take into account the continuity of $h_y$ and $\mu_0(h_z + m_z)$ on the interfaces and the Rado-Weertman boundary condition [4]. Using these conditions and replacing $s_y|k_y|$ with $k_y$ we obtain:

$$\begin{cases} \sum_j h_{0zj}\dfrac{|k_y|}{k_{zj}}\exp\left(-ik_{zj}L\right) = ih_{0z1}^e\exp\left(-|k_y|L\right) - ih_{0z2}^e\exp\left(|k_y|L\right), \\ \sum_j h_{0zj}\left(1 + \chi_{zzj}\right)\exp\left(-ik_{zj}L\right) = h_{0z1}^e\exp\left(-|k_y|L\right) + h_{0z2}^e\exp\left(|k_y|L\right), \\ \sum_j h_{0zj}\left(1 \pm i\xi k_{zj}\right)\chi_{zzj}\exp\left(-ik_{zj}L\right) = 0, \\ \sum_j h_{0zj}\left(1 \pm i\zeta k_{zj}\right)\chi_{yzj}\exp\left(-ik_{zj}L\right) = 0, \end{cases}$$

where

$$\chi_{yzj} = M_S\frac{\dfrac{k_y}{k_{zj}}\left[\dfrac{2A}{\mu_0 M_S}\left({k_y}^2 + {k_{zj}}^2\right) + H_{eff}\right] + \dfrac{i\omega}{|\gamma|\mu_0}}{\left[\dfrac{2A}{\mu_0 M_S}\left({k_y}^2 + {k_{zj}}^2\right) + H_{eff}\right]^2 - \dfrac{\omega^2}{\gamma^2{\mu_0}^2}}, \tag{S.6}$$

$$\chi_{zzj} = M_S\frac{\dfrac{2A}{\mu_0 M_S}\left({k_y}^2 + {k_{zj}}^2\right) + H_{eff} - \dfrac{k_y}{k_{zj}}\dfrac{i\omega}{|\gamma|\mu_0}}{\left[\dfrac{2A}{\mu_0 M_S}\left({k_y}^2 + {k_{zj}}^2\right) + H_{eff}\right]^2 - \dfrac{\omega^2}{\gamma^2{\mu_0}^2}}$$

$h_{0zj}$ and $h^e_{0z1,\ 2}$ here is the z-component of dynamic part of dipole field for $k_{zj}$ inside and outside the film, respectively, $L$ is z-coordinate of interface. The upper and lower signs in the formulas correspond to the upper and lower surfaces of the ferromagnetic layer, respectively. The quantities $\xi$ and $\zeta$ are introduced by analogy with the consideration of spin pinning at layer boundaries in [5] and can take values from 0 (fully pinned spins) to $\pm\infty$ (completely free spins) in directions perpendicular and parallel to the film plane (see details below), respectively. $h^e_{0z2} = 0$ for upper interface of all structure, $h^e_{0z1} = 0$ – for lower one.

To determine the frequencies for certain values of the $k_y$, we numerically vary the $\omega$ in (S.5 and S.6) to obtain zero determinant for systems (S.6) for all interfaces of structure [2, 3].

## II. ACCOUNTING FOR MAGNETOCRYSTALLINE AND SURFACE ANISOTROPY

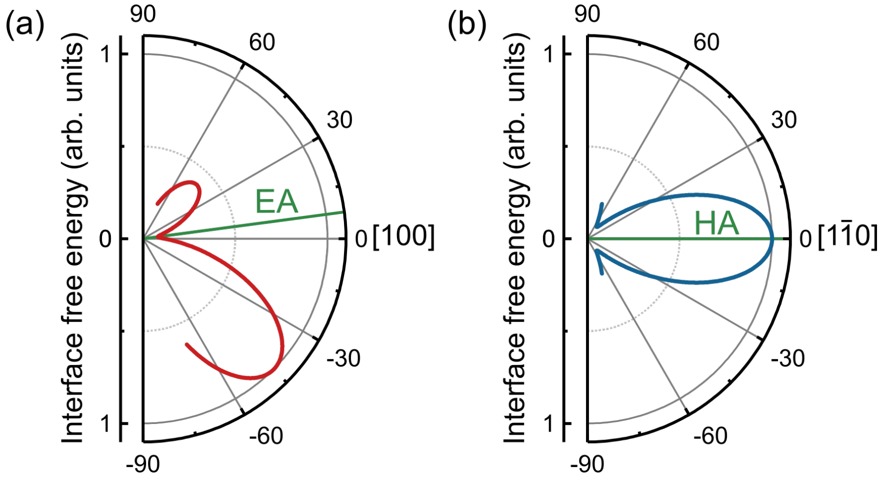


FIG. S.1. Free energy density around easy (a) and hard (b) magnetization directions.

The anisotropy energy for the structures under investigation is written as [6]:

$$U_A = \frac{K_C}{4}\left[\sin^4\theta\sin^2 2\phi + \sin^2 2\theta\right] - \frac{K_U}{2}\sin 2\phi\sin^2\theta, \tag{S.7}$$

where $\phi$ and $\theta$ is the azimuthal and polar angles of $\mathbf{M}$, $K_C$ and $K_U$ – first order cubic and uniaxial anisotropy parameters, respectively.

In the case of in-plane external magnetic field, $\theta$ is always equal to $\pi/2$. To determine the orientation of EA and HA we can differentiate (S.7) with respect to $\phi$. For a condition to energy extremum positions we obtain:

$$\cos 2\phi \left(K_C \sin 2\phi - K_U\right), \tag{S.8}$$

where the first multiplier determines the position of HA, while the second one - position of EA.

The position of HA from (S.8) coincides with direction $[1\bar{1}0]$. The position of EA is close to [100] direction and tilted by an angle $1/2 \arcsin K_U/K_C$ which is, in our case, about $7^\circ$ (see Fig. S.1). In the experiments we use direction [100] as an EA. The corresponding anisotropy field for magnetization along easy and hard axis is 0 and $-\frac{K_C - K_U}{\mu_0 M_S}$, respectively [7].

## III. PINNING PARAMETERS AND METHOD FOR CALCULATING THE AMPLITUDES DISTRIBUTION OVER THE THICKNESS OF THE STRUCTURE

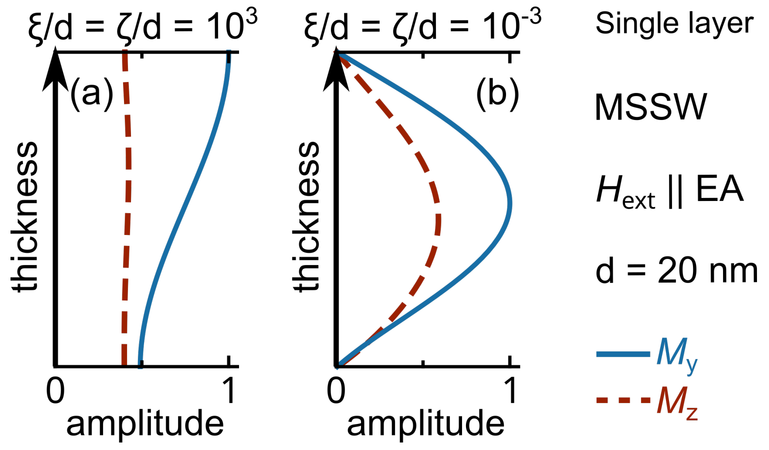


FIG. S.2. Distributions of the amplitudes of in-plane $M_y$ and out-of-plane $M_z$ magnetization components over the thickness of the single layer in the case close to fully free (a) and fully pinned (b) condition. The data were obtained for the MSSW at $k_y = 22 \cdot 10^4$ rad/cm.

No additional anisotropy axes are expected at the interfaces under consideration [8]. As a pinning conditions we consider changes in values of volume exchange stiffness and anisotropy parameters at the interfaces. Thus, in accordance with [9], the surface anisotropy for the films under study is written in a form similar to (S.7).

We used boundary conditions in the form of pinning parameters because of their clear physical meaning (see Fig. S.2). The values of $\xi$ and $\zeta$ demonstrate the behavior of the amplitudes at the interfaces from the zero amplitude to the zero value of its first derivative

with respect to the coordinate perpendicular to the layer [5]. Using surface anisotropy energy in the form (S.7) we obtain pinning parameters values $\xi = -\frac{2A}{K_C^{surf} + K_U^{surf}}$ and $\zeta = \frac{A}{K_C^{surf} - K_U^{surf}}$ when **M** and **H** along $[1\bar{1}0]$. Along [100] direction we obtain $\xi = -\frac{A}{K_C^{surf}}$ and $\zeta = \frac{AK_C^{surf}}{(K_U^{surf})^2 - (K_C^{surf})^2}$. In the fitting process, the pinning parameters for EA and HA were selected in such a way as to correspond to the same values of $K_C^{surf}$ and $K_U^{surf}$.

Thickness distribution of $M_y$ and $M_z$ for certain values of the $k_y$ and $\omega$ was obtained using $h_{0zj}$ and $\chi_{yzj}$, $\chi_{zzj}$ from (S.6). Since the determinant of the system of equations (S.6) is equal to zero, there is a non-trivial solution, which was found numerically. Next we can calculate distribution of $h_{0z}$ fields as function of amplitude one of the $h^e_{0z1,\ 2}$ fields and using $\chi_{yzj}$ and $\chi_{zzj}$ obtain $M_y$ and $M_z$ dependencies. We use for one of the $h^e_{0z1,\ 2}$ fields value $E^{i\phi}$ and vary $\phi$ in order to achieve the amplitude value for $M_y$ and $M_z$. As expected, the $\phi$ values for the two components differed by $\pi/2$.

## IV. SURFACE MAGNETOSTATIC WAVES WITHOUT INTERLAYER COUPLING

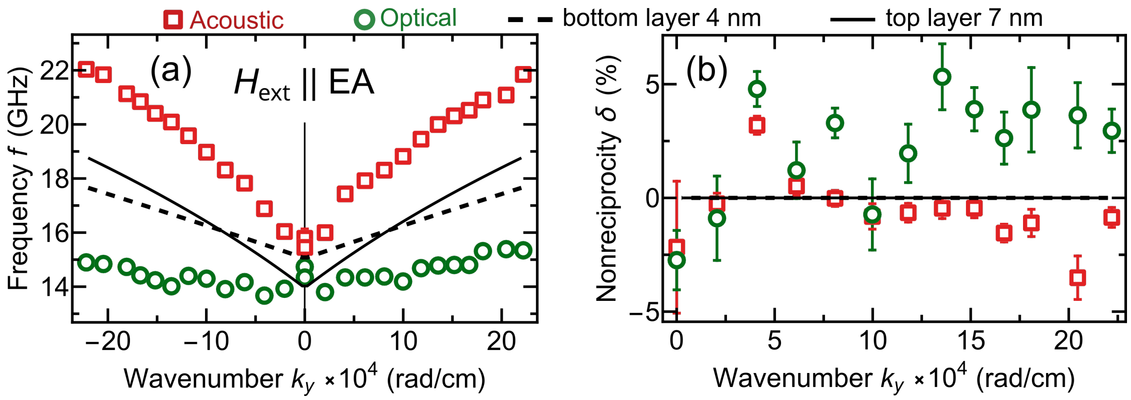


FIG. S.3. (a) dispersion of MSWs in a bilayer structure, obtained from the BLS experiments (points) and (b) nonreciprocity vs $k_y$ for data from (a) using (S.9). $\mathbf{H}_{\text{ext}}$ applied along EA. The lines show numerical solution using the (S.6) model for single 4 nm (dashed line) and 7 nm (solid line) layers.

Fig. S.3 a show the experimental dispersion of MSWs in multilayered system. Two branches are visible. One of the branches exhibits a behavior similar to the surface mag-

netostatic spin wave (MSSW). The second branch is observed at lower frequencies than the MSSWs for both ferromagnetic layers and demonstrates a weak dependence on $k_y$ in the entire investigated range. The lines in the Fig. S.3 shows the results of the model for isolated layers with a thickness of 7 (solid line) and 4 nm (dashed line). In this case, both observed in the experiment branches cannot be described in terms of single layer models at any pinning parameters values. In addition, single layer models do not predict nonreciprocity observed in the experiment for nonzero values of $k_y$ (see Fig. S.3 b). Thus, we come to the conclusion that the observed dispersion refers to collective modes of spin waves in a multilayer structure.

## V. NONRECIPROCITY CALCULATION DETAILS

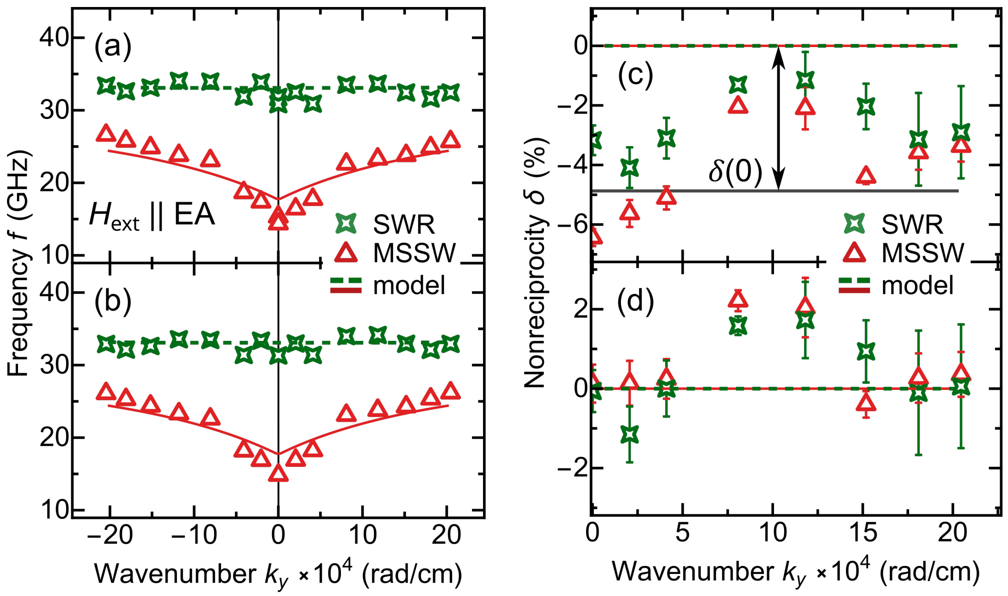


FIG. S.4. Thermal magnons dispersions in single galfenol film for $\mathbf{H}_{ext}$ applied along easy magnetization direction (a) before and (b) after correction (see details in the text). Lines show the best fit of experimental data using model Eq. S.9. Nonreciprocity of MSWs (c) before correction [using data from (a)] and (d) after correction [using data from (b)]. Solid black line represent $\delta(0)$.

To quantify the nonreciprocity, we introduce the dimensionless parameter:

$$\delta(k_y) = 2[f(k_y) - f(-k_y)]/[f(k_y) + f(-k_y)]. \tag{S.9}$$

There is a k-vector-independent component $\delta(0) \neq 0$ for multilayer structure and single film under experiment (see Fig. S.4 c). This component can be explained by additional minor peaks that are unresolvable in the experiment with different intensities in the Stokes and anti-Stokes parts of the spectrum, which make up broad peaks in the BLS spectra (full width at half maximum of all experimental peaks is around 1.5 GHz). When described by a single Lorentz peak, such a set of peaks leads to a different shift of the center frequency for $k_y > 0$ and $k_y < 0$. These minor peaks may originate from spin wave modes with close frequencies emerging due to the gradients of the magnetic parameters of the ferromagnetic layers near the interfaces [10]. The shift in the frequency of the entire group of peaks with a $k_y$ change leads to a wavenumber-independent contribution to the nonreciprocity. The uncertanty in determining the center frequency of the peak $\Delta f$ is determined as the difference between the frequencies of the Stokes and anti-Stokes peaks $< f_{Stokes} - f_{anti-Stokes} >_{MSSW,SWR}$ of a single galfenol film at $k_y = 0$ and an external magnetic field along EA. The dispersion dependencies of a single galfenol film magnetized along EA before and after correction are shown in Fig. S.4 a and b, respectively. This correction was introduced for all experimental results. After correction the nonreciprocity for single film is $\delta(k_y) = 0$ which agrees with the model results (see Fig. S.4 d). The same correction value was introduced into the data for the bilayered structure. In the main text, only the wavevector-dependent nonreciprocity $\delta(k_y)$ is discussed. Since for a single layer the numerical solution does not demonstrate nonreciprocity (see Fig. S.4 c,d), in the case of a bilayer structure, the nonreciprocity predicted by the model is associated with the dipole interaction between the ferromagnetic layers.

## VI. PINNING PARAMETERS AT THE INTERFACES WITH A COPPER INTERLAYER

Since there are no interfaces between the ferromagnetic layer and copper in the investigated single galfenol film, the pinning parameters on such an interface of the double layer structure may differ from the film/air and film/substrate values. Since no additional anisotropy axes associated with the interfaces are expected for all interfaces of the structure under study [11], we assume only slightly different pinning parameters at the interfaces with copper interlayer. Figures S.5 (a) and (b) show the dispersion and dependence of the frequency nonreciprocity on $k_y$ for the structure ($d_b$ =4 nm, $d_t$ =7 nm) with the same magnetic

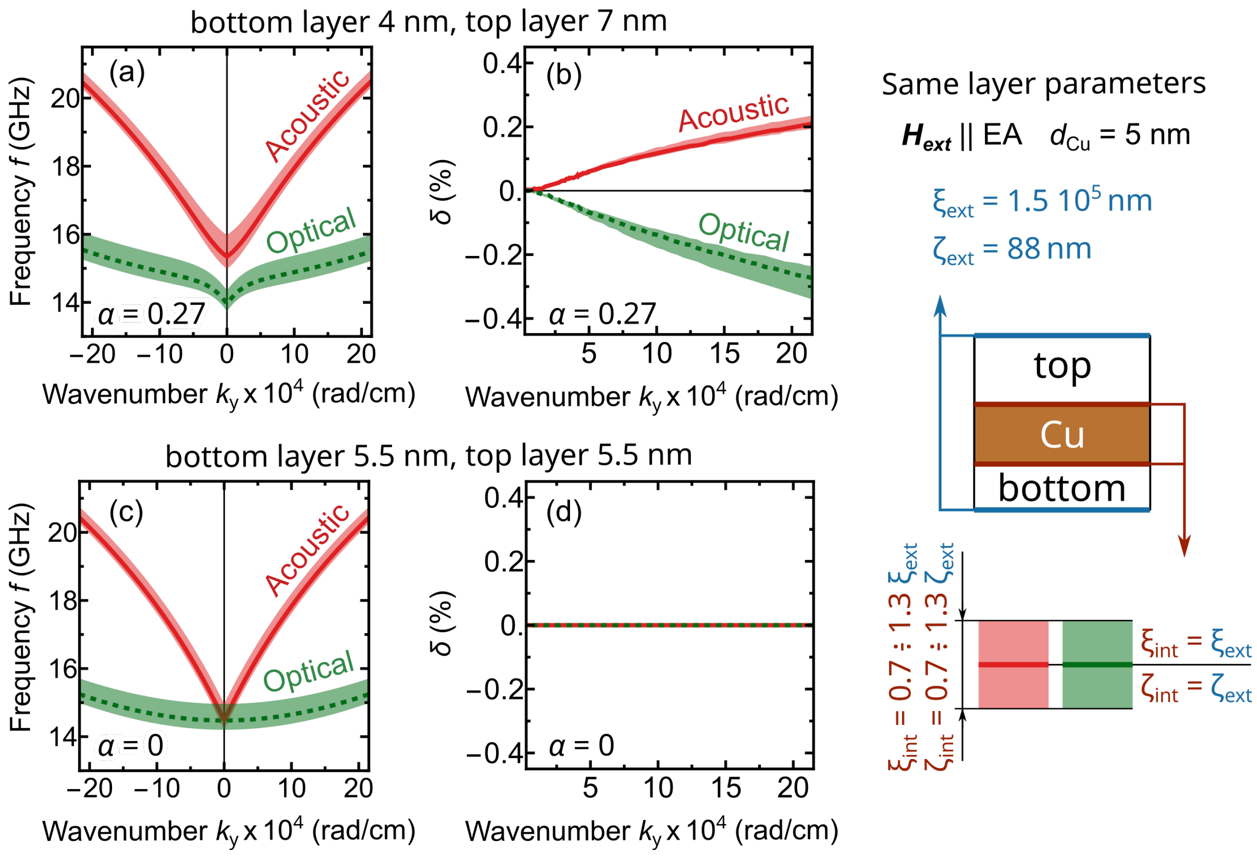


FIG. S.5. MSWs dispersion calculated by the model for the ferromagnetic layers thicknesses of the structure under experiment (a) and the geometrically symmetric double layer (c). (b) and (d) corresponding nonreciprocity of dispersions from (a) and (c), respectively. The calculations was performed for the same values of the magnetic parameters of the top and bottom layers. The lines show the values at the same pinning parameters at the edges of the entire structure and at interfaces with a copper interlayer. The shaded areas show the change in the values when varying the pinning parameters at the interfaces with the copper layer in the range 70 - 130%.

parameters of the layers, respectively. The shaded areas show the change in the simulated values when varying the pinning parameters on the interfaces with copper in the range from -30 to +30 % (see the explanatory diagram in the Fig. S.5). It can be seen that a change in the pinning parameters leads to a quantitative change in the values. However, as demonstrate the simulation results for a structure with equal ferromagnetic layers thicknesses (Fig. S.5 (c,d)), a change in pinning at interfaces with copper does not in itself lead to nonreciprocity. The dependences of nonreciprocity on the geometric asymmetry of the structure for all values of the pinning parameters in the investigated range qualitatively

repeat the dependences in figures 2 (a) and (b) in the article text.

## VII. NONRECIPROCITY IN THE CASE OF DIFFERENT MAGNETIC PARAMETERS OF THE LAYERS

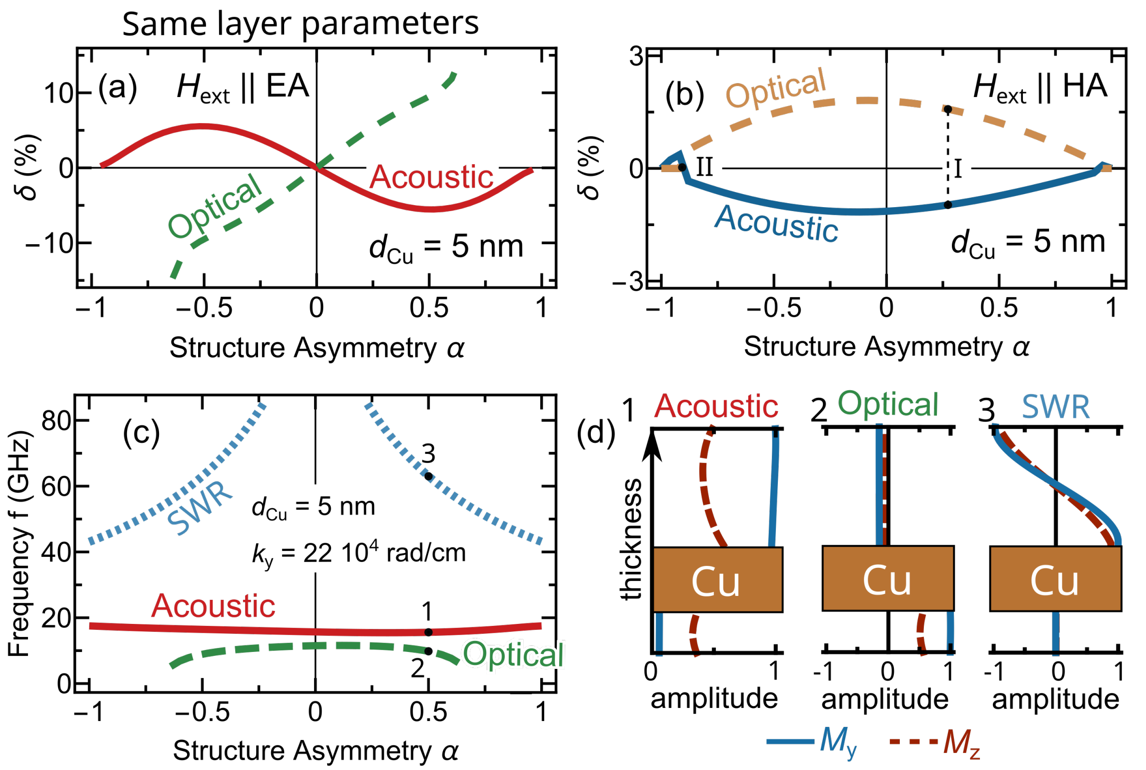


FIG. S.6. Nonreciprocity parameter $\delta$ from the model vs structure asymmetry $\alpha$ (a) for the case of the same layer parameters ($\mu_0 M_S = 1.7\,\mathrm{T}$ and $\mathbf{H_{eff}} = \mathbf{H_{ext}}||$ EA) and (b) for the structure under experiment with an external field along HA. (c) the frequencies of magnetization dynamics vs structure asymmetry for structure from (a) at $k_y = 22 \cdot 10^4\,\mathrm{rad/cm}$. (d) distributions of the amplitudes of in-plane $M_y$ and out-of-plane $M_z$ magnetization components over the thickness of the structure for acoustic (point 1 in panel (c)), optical (point 2), and PSSW (point 3) branches.

In the case of identical magnetic parameters of two ferromagnetic layers (saturation magnetization and anisotropy parameters), the absolute values of nonreciprocity are symmetric about the point $\alpha = 0$ where $\delta(k_y)$ vanishes (Fig. S.6 a). In the case when the magnetic parameters of the ferromagnetic layers differ, nonzero nonreciprocity occurs for a geometrically symmetric system (see Fig. S.6 b and Fig. 2 a in the article). Fig. S.6 b shows the

dependence $\delta(\alpha)$ for both modes at $|k_y| = 22 \cdot 10^4$ rad/cm, $d_{Cu} = 5$ nm, and $\mathbf{H_{ext}}$ directed along HA. In the case of $\delta(0) \neq 0$ and $\alpha \neq 0$ the nonreciprocity can be either increased or suppressed, depending on the geometric asymmetry of the structure.

## VIII. SPIN WAVE MODES IN THE CASE OF $\alpha \to \pm 1$

The dependences of $\delta(\alpha)$ are given in the range of simultaneously existing acoustic and optical dispersive branches of magnetostatic waves. When approaching the case of a single film, i.e. to the values $\alpha = \pm 1$, a transition is observed from the collective dynamics of the magnetization of two dipole-coupled ferromagnetic layers to the propagation of surface wave and SWR in a single film. Fig. S.6 c shows the dependencies of the magnetic dynamics frequencies on the geometric asymmetry for waves propagating in the positive direction at $k_y = 22 \cdot 10^4$ rad/cm. For strongly asymmetric structures, the model predicts the appearance of a third dispersion branch in the investigated frequency range. In contrast to the acoustic (point 1) and optical (point 2) modes, the SWR branch is observed (point 3) with a nonzero amplitude only in a thicker layer (see Fig. S.6 d). This branch refers to the magnetization dynamics in only one of the layers and does not participate in the formation of collective modes. The branch of collective dynamics, which coincides in frequency with the surface wave at $\alpha \to \pm 1$, is transformed into the MSSW.

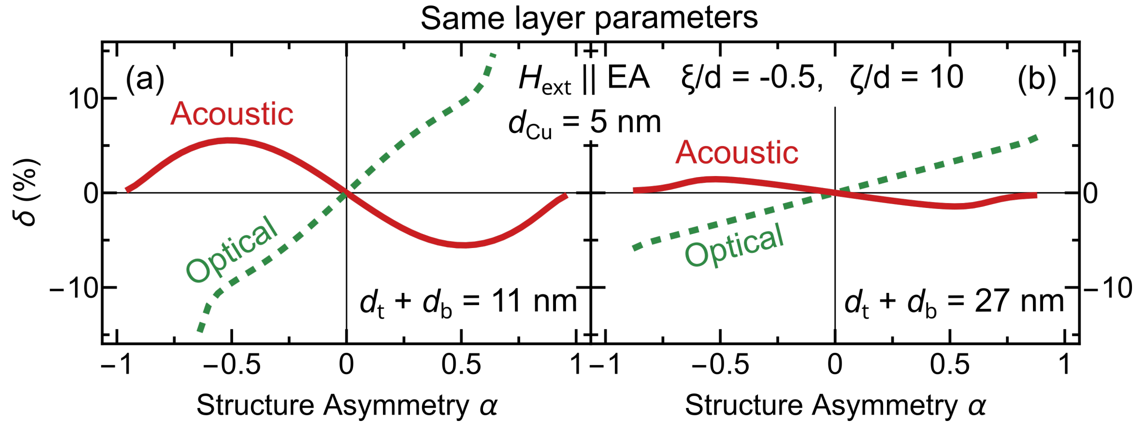


FIG. S.7. Nonreciprocity parameter $\delta$ from the model vs structure asymmetry $\alpha$ for the case of the same layer parameters with an external field along EA at $\xi = -0.5$ nm and $\zeta = 10$ for two values of total thickness $d_t + d_b = 11$ (a) and 27 nm (b).

## IX. EFFECT OF TOTAL THICKNESS OF TWO FERROMAGNETIC LAYERS ON NONRECIPROCITY

Fig. S.7 show the nonreciprocity vs structure asymmetry for bilayers with different total thickness of two ferromagnetic layers. The decreasing in nonreciprocity with increasing of total thickness is clearly seen. With a further increase in the thickness, it becomes difficult to determine the nonreciprocity due to the intersection of the SWR and Acoustic branches.

---


[1] G. Rado and R. Hicken, Theory of magnetic surface anisotropy and exchange effects in the Brillouin scattering of light by magnetostatic spin waves, Journal of Applied Physics **63**, 3885 (1988).

[2] B. Hillebrands, Spin-wave calculations for multilayered structures, Physical Review B **41**, 530 (1990).

[3] G. Carlotti and G. Gubbiotti, Brillouin scattering and magnetic excitations in layered structures, La Rivista del Nuovo Cimento (1978-1999) **22**, 1 (1999).

[4] G. T. Rado and J. R. Weertman, Spin-wave resonance in a ferromagnetic metal, Journal of Physics and chemistry of solids **11**, 315 (1959).

[5] A. G. Gurevich and G. A. Melkov, *Magnetization oscillations and waves* (CRC press, 1996).

[6] N. E. Khokhlov, P. I. Gerevenkov, L. A. Shelukhin, A. V. Azovtsev, N. A. Pertsev, M. Wang, A. W. Rushforth, A. V. Scherbakov, and A. M. Kalashnikova, Optical excitation of propagating magnetostatic waves in an epitaxial galfenol film by ultrafast magnetic anisotropy change, Physical Review Applied **12**, 044044 (2019).

[7] S. Chikazumi, *Physics of Ferromagnetism*, International Series of Monographs on Physics (OUP Oxford, 2009).

[8] B. Dieny and M. Chshiev, Perpendicular magnetic anisotropy at transition metal/oxide interfaces and applications, Reviews of Modern Physics **89**, 025008 (2017).

[9] G. Wastlbauer and J. A. C. Bland, Structural and magnetic properties of ultrathin epitaxial fe films on gaas (001) and related semiconductor substrates, Advances in physics **54**, 137 (2005).

[10] C. Vaz, J. Bland, and G. Lauhoff, Magnetism in ultrathin film structures, Reports on Progress in Physics **71**, 056501 (2008).

[11] B. Dieny and M. Chshiev, Perpendicular magnetic anisotropy at transition metal/oxide interfaces and applications, Rev. Mod. Phys. **89**, 025008 (2017).
